# Supplementary material for: Towards Better Explanations for Object Detection
Source: arXiv:2306.02744 source file (2023-06-06)
Supplement: Supplementary file 1 [file appendix.tex]

\appendix
\label{sec:appendix}

% \section{}
